# Supplementary material for: Towards Efficient and Domain-Agnostic Evasion Attack with High-dimensional Categorical Inputs
Source: arXiv:2212.06836 source file (2022-12-13)
Supplement: Supplementary file 1 [file Appendix_5_RadorFigure_Analysis.tex]

\section{Radar charts over EHR and IPS dataset}
We provide the radar charts of all the involved attack methods in the experimental study over EHR and IPS data respectively in Figure.5.

\begin{figure}[t]\label{Appendixfig:RadorFig}
% \small
\centering
\begin{minipage}[t]{0.33\linewidth}
\centering
\includegraphics[width=\textwidth]{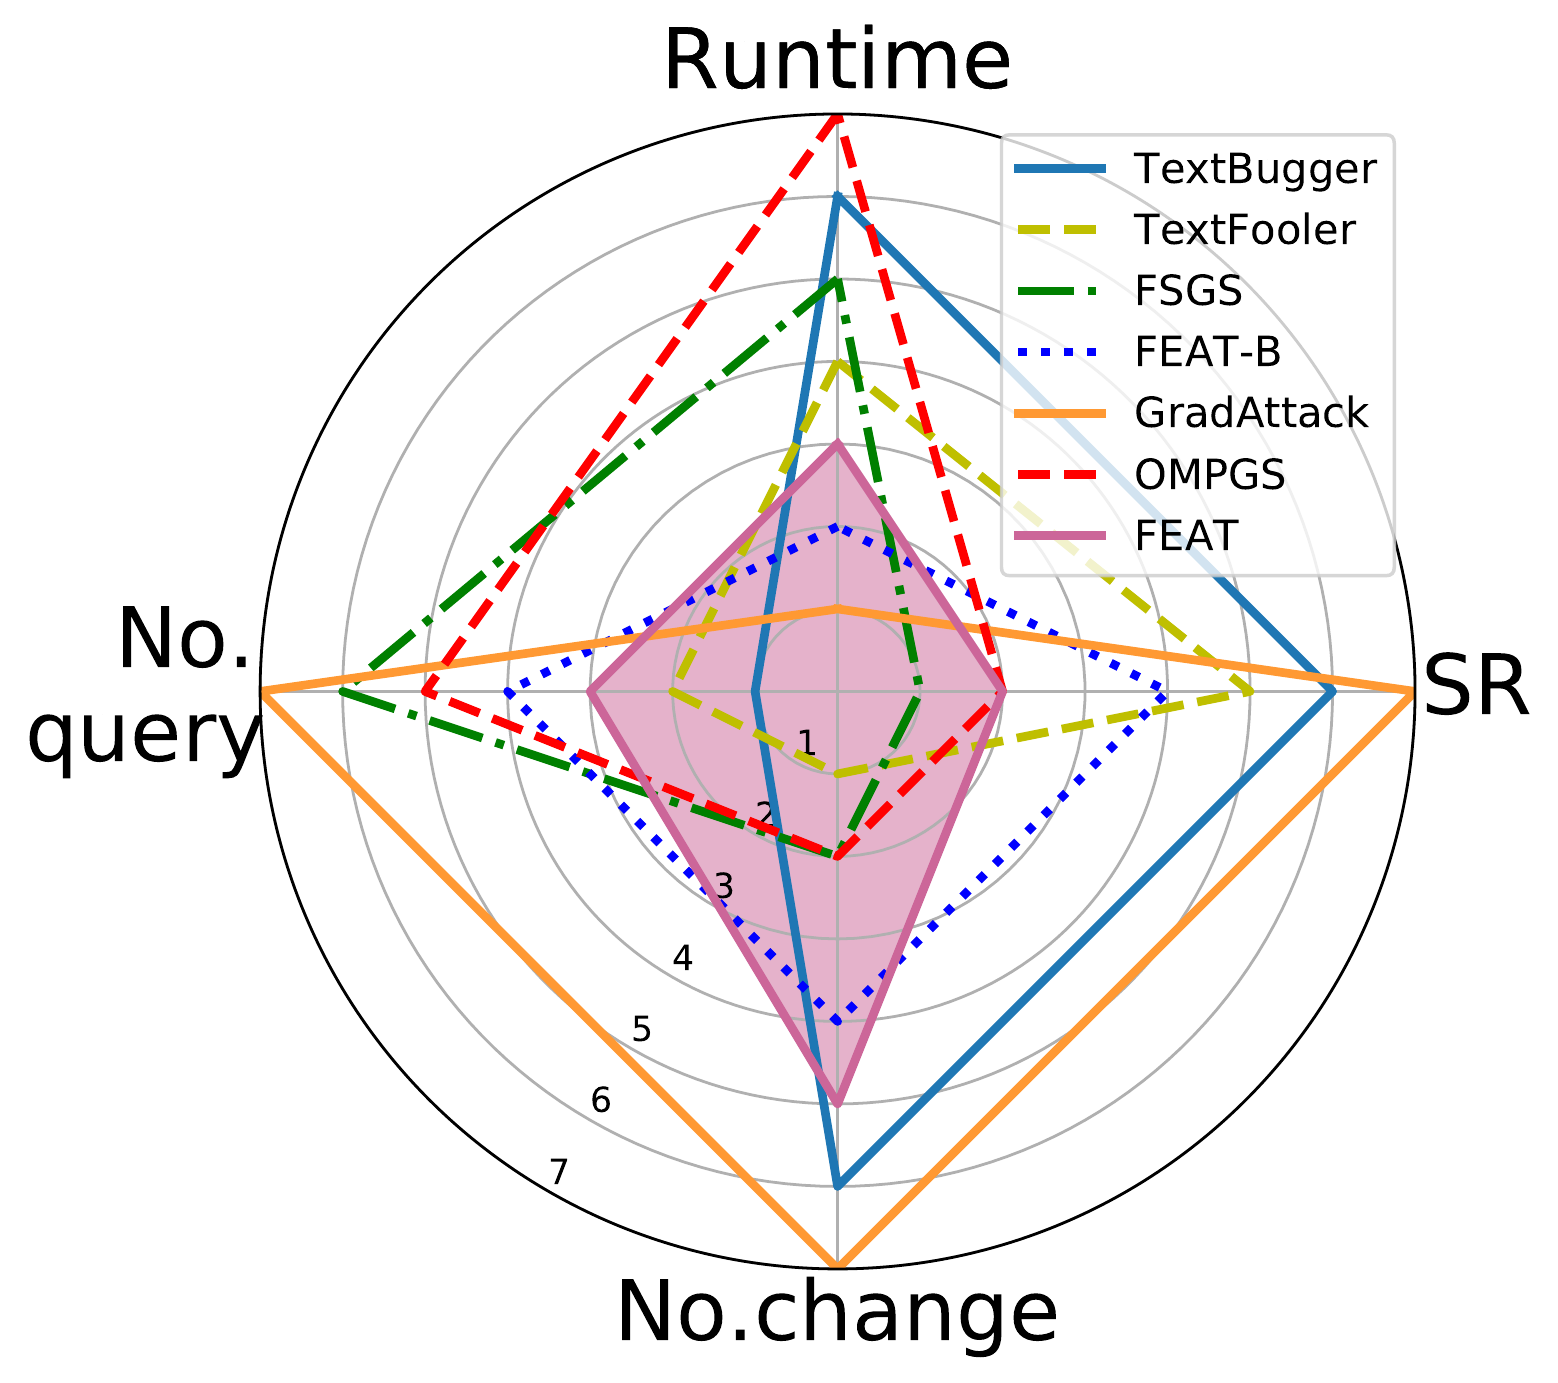}\\
% \vspace{-0.2cm}
{\scriptsize (a) Yelp-5, attack budget=10}
\end{minipage}%
\hspace{10mm}
\begin{minipage}[t]{0.33\linewidth}
\centering
\includegraphics[width=\textwidth]{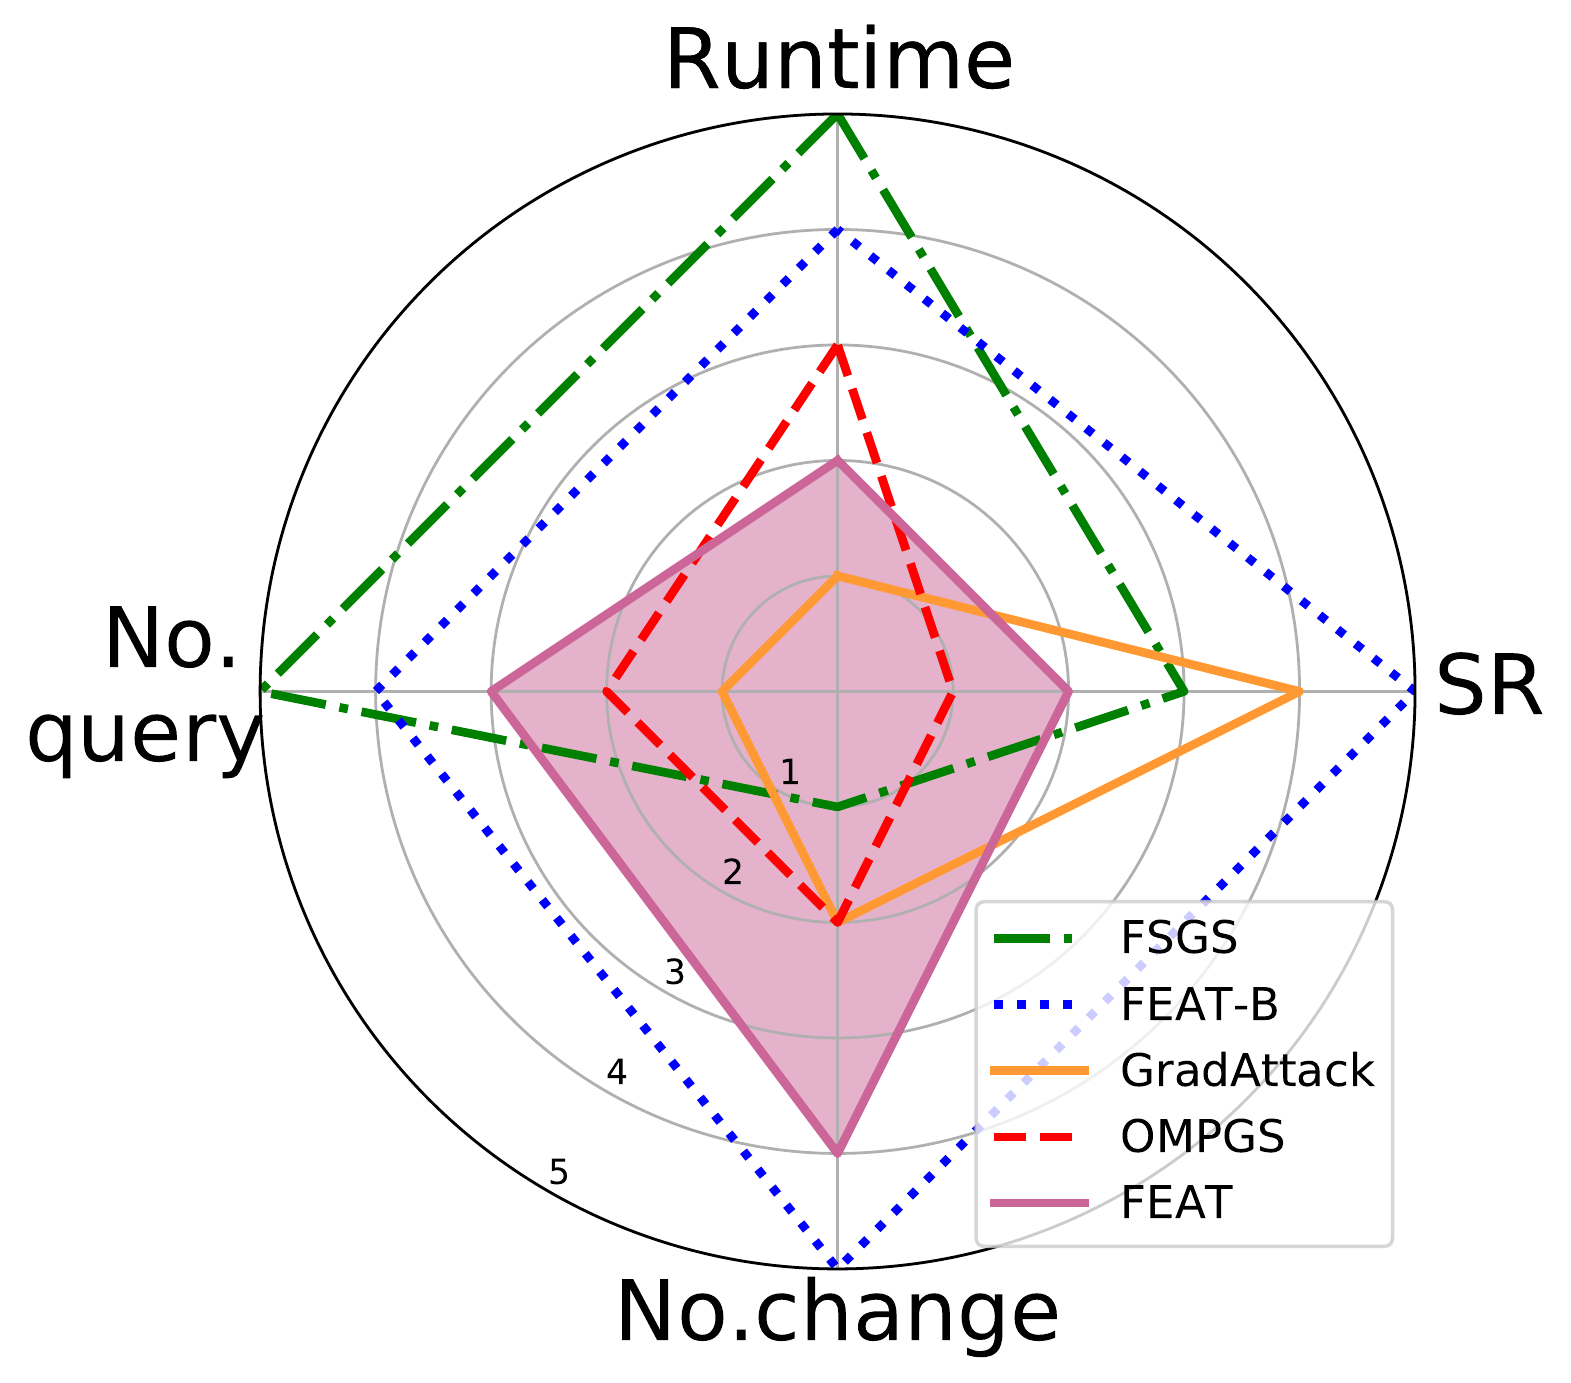}\\
% \vspace{-0.2cm}
{\scriptsize (b) EHR, attack budget=4}
%\caption{fig2}
\end{minipage}%
\caption{Comparison of attack performance ranked by AT, AE, AC and SR on Yelp-5 and EHR. The best attack method ranked the 1st is located at the first ring. }
%\vspace{-0.6cm}
\end{figure}

%\begin{figure}[t]\label{fig:features_sensitivity}
% \small
%\centering
%\begin{minipage}[t]{0.25\linewidth}
%\centering
%\includegraphics[width=\textwidth]{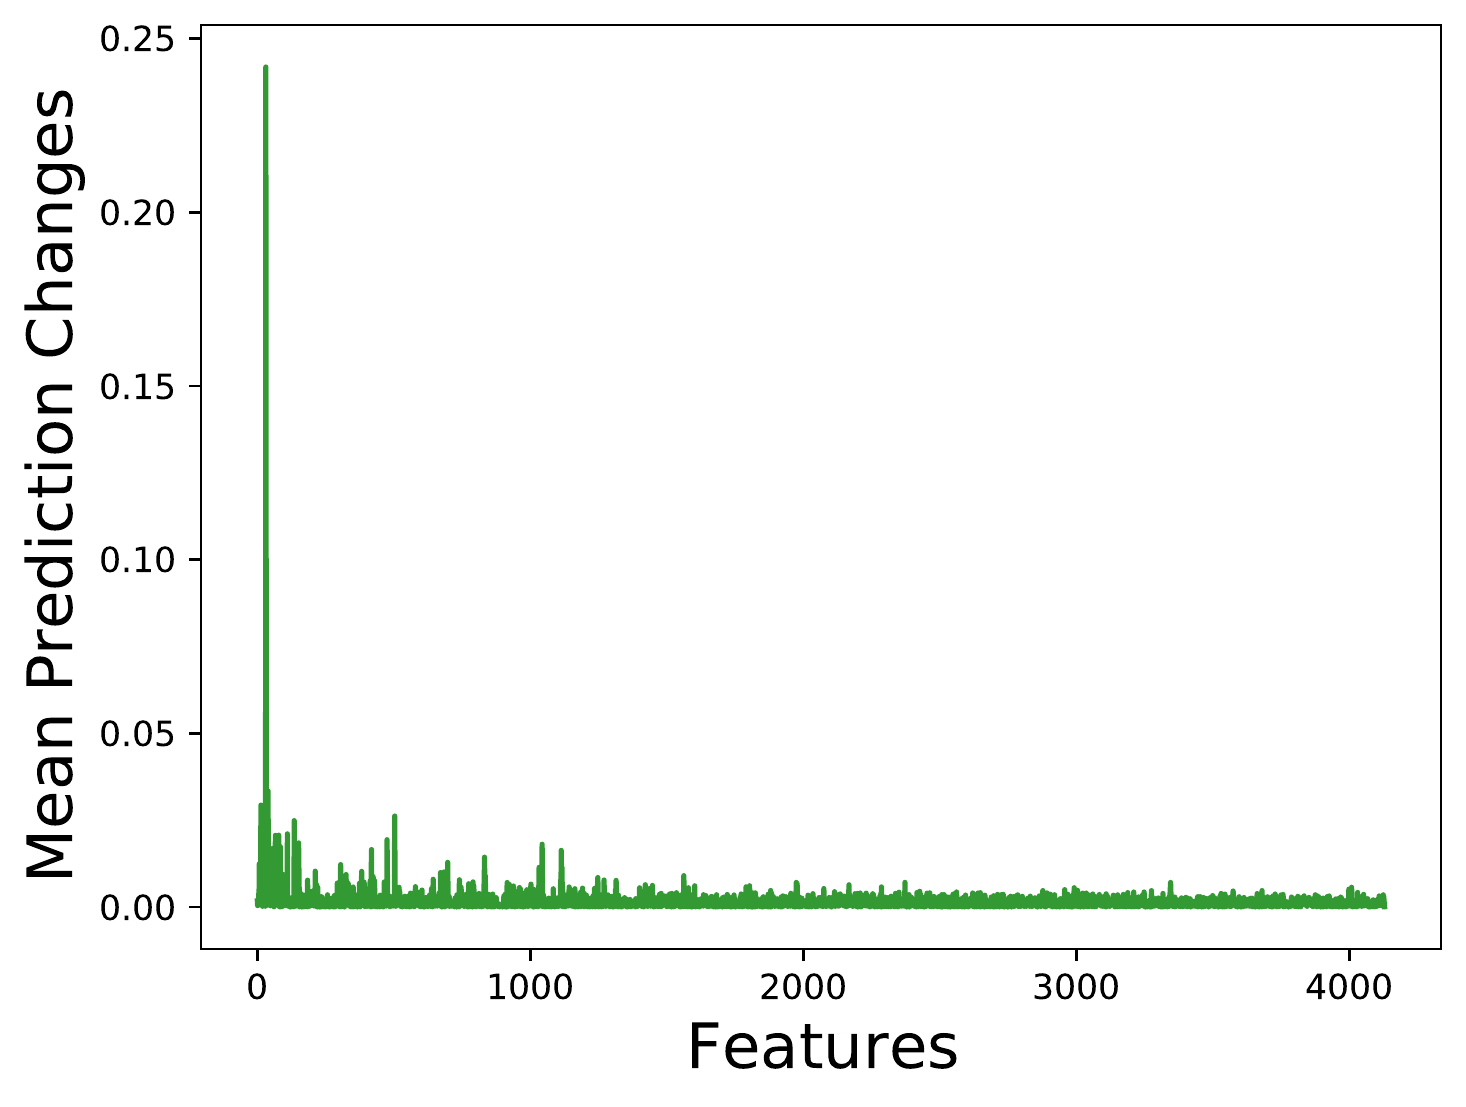}\\
%\vspace{-0.25cm}
%{\scriptsize (a)EHR, attack budget=10}
%\end{minipage}%
%\hspace{5mm}
%\begin{minipage}[t]{0.25\linewidth}
%\centering
%\includegraphics[width=\textwidth]{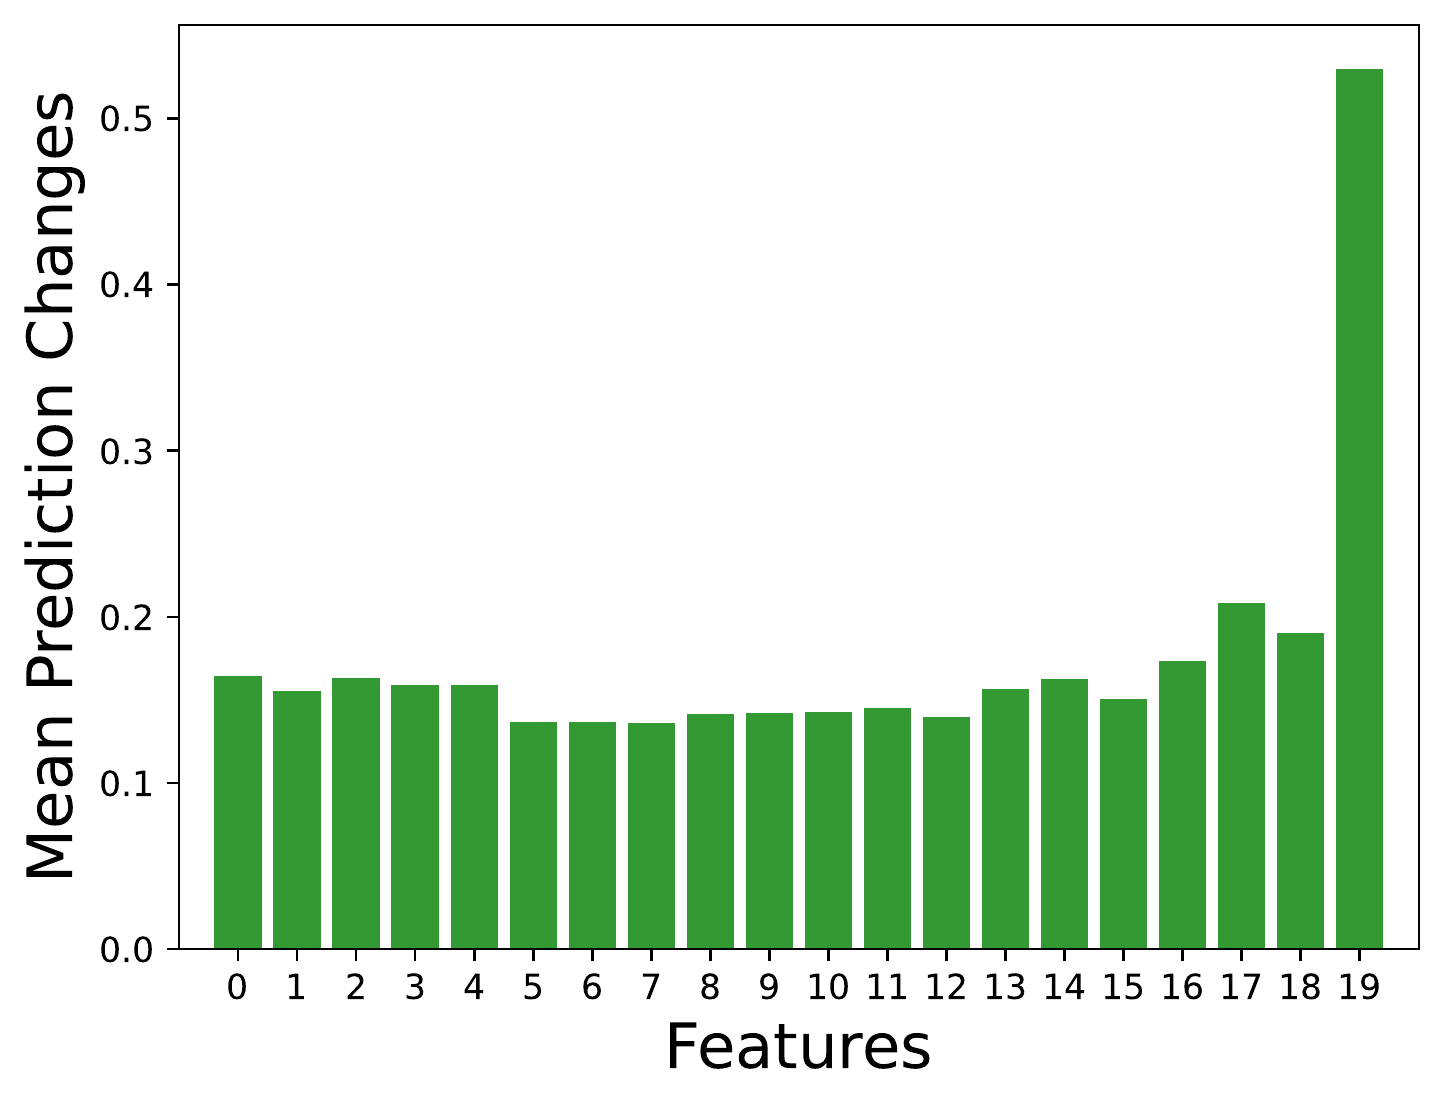}\\
%\vspace{-0.25cm}
%{\scriptsize (b) IPS, attack budget=4}
%\caption{fig2}
%\end{minipage}%
%\hspace{5mm}
%\begin{minipage}[t]{0.25\linewidth}
%\centering
%\includegraphics[width=\textwidth]{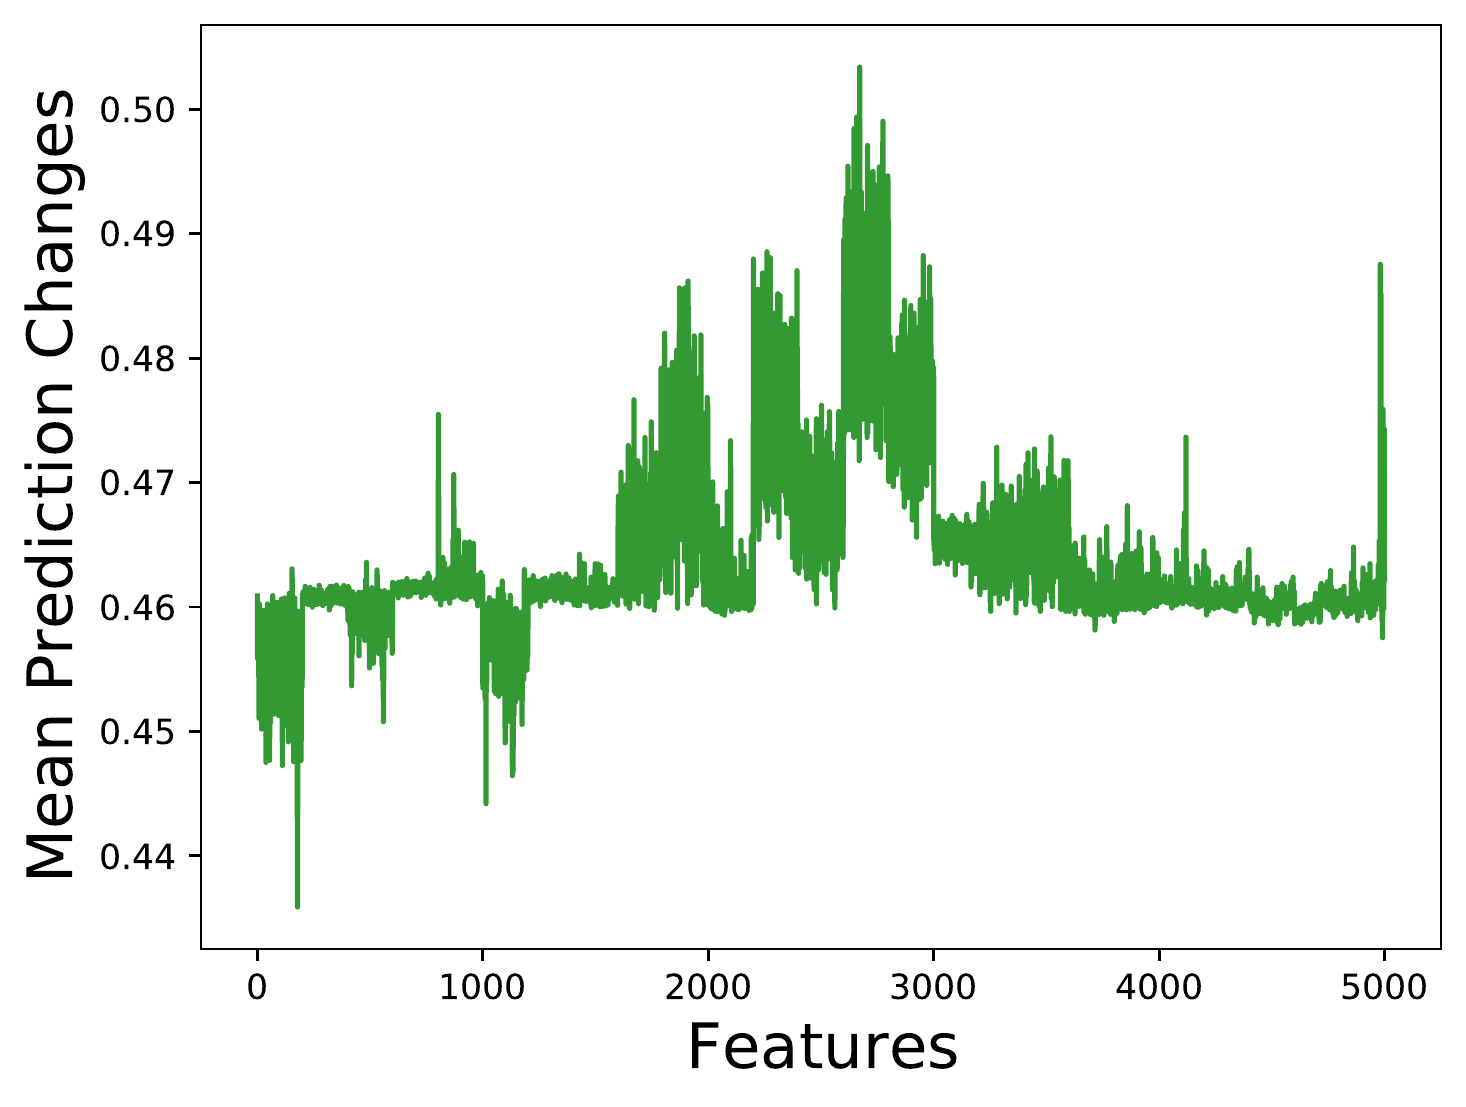}\\
%\vspace{-0.25cm}
%{\scriptsize (c) PEDec}
%\caption{fig2}
%\end{minipage}

%\caption{Comparison of feature sensitivity on EHR, IPS and PEDec. }
%\vspace{-0.6cm}
%\end{figure}
